# Supplementary material for: WHAC: World-grounded Humans and Cameras
Source: arXiv:2403.12959 source file (2024-03-19)
Supplement: Supplementary file 1 [file 9_supp.tex]

hyperparameters (GRU, MV)
MV architecture
adaptation of smpler-x and osx
inference speed
more visualization 
- emdb: trajectory
- whac-a-mole: trajectory + overlay
